# Supplementary material for: Generalized Bond Polarizability model for more accurate atomistic modeling of Raman spectra
Source: arXiv:2501.12059 source file (2025-01-21)
Supplement: Supplementary file 1 [file supplementary_materials.pdf]

# Supplementary Material for Generalized Bond Polarizability model for more accurate atomistic modeling of Raman spectra

Atanu Paul,[1] Nagaprasad Reddy Samala,[1] and Ilya Grinberg[1]
*Department of Chemistry, Bar-Ilan University, Ramat Gan 5290002, Israel*

(*ilya.grinberg@biu.ac.il)

### A. Results of $SO_2$, $H_2S$, $CH_4$ and $NH_3$

Results of BPM and GBPM in comparison with DFPT in case of $SO_2$, $H_2S$ and $CH_4$ are shown in Fig. S1, S2 and S3, respectively. Fig. S4 shows the value of $\alpha$ for $NH_3$ calculated using BPM and GBPM with that calculated using DFPT. The triangular-shape like data distribution of $\alpha$ (e.g. $\alpha_{xx}$, $\alpha_{yy}$, $\alpha_{zz}$) of the BPM results can be visualized in the plot.

TABLE I. $R^2$ value of $\alpha_{xx}$ calculated using BPM and GBPM model for the respective systems

| | BPM | GBPM |
|---|---|---|
| $H_2O$ | 0.2437 | 0.9991 |
| $NH_3$ | 0.9984 | 0.9998 |
| $CH_3OH$ | 0.9781 | 0.9929 |
| $CH_3CH_2OH$ | 0.9769 | 0.9829 |
| $BaTiO_3$ | 0.6169 | 0.8941 |

### B. The coefficient of determination, or $R^2$ value

$R^2$ values of $\alpha_{xx}$ from BPM and GBPM models for the studied systems (see Table I) are calculated using the following expression:

$$R^2 = 1 - \frac{\sum(\alpha_{xx}^{DFPT} - \alpha_{xx}^{Model})^2}{\sum(\alpha_{xx}^{DFPT} - \overline{\alpha_{xx}^{DFPT}})^2}$$

where $\alpha_{xx}^{DFPT}$ and $\alpha_{xx}^{Model}$ are the value of $\alpha_{xx}$ using DFPT and model (BPM, GBPM), respectively. $\overline{\alpha_{xx}^{DFPT}}$ is the average value of $\alpha_{xx}^{DFPT}$.

### C. Accuracy test for different level of GBPM in case of $CH_3OH$

Fig. S5 (a) and (b) compare the Raman spectra of $CH_3OH$ calculated using DFPT and different level of GBPM in lower and higher wavenumber region, respectively. Here, the result of GBPM containing the effect of BPM and bond H-C in H-O-C angle is represented by GBPM (BPM + H-O-C). Similarly, GBPM (BPM + H-C-H) contains the effect of BPM along with H-H bond in H-C-H angle. While including these two bonds (H-O-C and H-C-H) with BPM, the result is represented by GBPM (BPM + H-C-H + H-O-C). Finally, GBPM (BPM + H-C-H + H-O-C + H-C-O) contains all possible bonds formed by angle H-C-H, H-O-C, H-C-O along with BPM in $CH_3OH$.

### D. Convergence with number of structures for $H_2O$ and $CH_3OH$

To examine the convergence of the fitted polarizability models with respect to the number of structures in the training set used for fitting of polarizability models, we used 12, 24, and 36 H2O structures in the fitting of the models for $H_2O$. In Figs. S6 (a) and (b), we plot the values of $\alpha_{xx}$ calculated by the model along the DFT simulation trajectory (a total of 17312 structure) versus the corresponding values obtained by DFPT calculations. For BPM, it can be observed that the triangular shape-like data distribution is present for all cases and the distributed data cannot be aligned along the ideal $y = x$ line irrespective of the number of considered DFPT structures for the parametrization of the BPM. This discrepancy is due to the incompleteness of the BPM for modeling the electronic polarizability as discussed already in the manuscript. However, the triangular shape is converged for the 24 structures indicating that DFPT results of 24 structures are required to get a converged parameters for the BPM. In case of GBPM results (see Figs. S6 (b)), the distributed data for those three differnet number of structures are aligned along ideal y = x line. However, the data are scattered in case of 12 structures and become perfectly aligned for 24 structures, showing that inclusion of more structures in the training set no longer provide an improvement in the model quality. This means that the model is converged with respect to the number of the structures in the training set. Similar results are obtained for $CH_3OH$ where we use 36, 48 and 60 structures as shown in Figure S7. No differences in the scatter in the plot of DFT $\alpha_{xx}$ versus model $\alpha_{xx}$ are observed between the models obtained using 48 and 60 structures, and a slightly greater scatter is observed for the model obtained using 36 structures. The results show that for this molecule 48 structures are sufficient to obtain converged BPM and GBPM results.

### E. Results of first and second order GBPM for $H_2O$

Comparison of first and second order model of GBPM is presented in Fig. S8. Fig. S8 (a) shows the *xx* component of $\alpha$ calculated after considering first and second order terms of the Taylor series expansion of GBPM model along with that DFPT-calculated value of $\alpha$. The polarizability trajectory of these different methods can be visualized in Fig. S8 (b). The

Raman spectra as calculated using the polarizability trajectory for these different methods are shown in Fig. S8 (c). From all these results it is evident that similar to second-order-GBPM, first-order-GBPM model which consider only eight parameters is also capable to reproduce the DFPT results accurately for $H_2O$.

### F. O-O interactions in the GBPM model for $BaTiO_3$

The plot of the maximally localized Wannier function of the O-$p$ orbital in rhombohedral $BaTiO_3$ presented in Fig. S9 shows that there are states that connect the two O atoms forming a 90° O-Ti-O angle (O atoms O1 and O2 in the figure). Additionally there is significant charge density located along the line connecting these two O atoms. These states are due to the lone pair O orbitals which provide the top of the valence band of $BaTiO_3$ and thus are important for polarizability. It is clear that changes in the distance between O atoms O1 and O2 will affect the shape of the charge density and therefore the polarizability of the $BaTiO_3$. This is due to the changes in the quantum mechanical orbital overlap covalent interactions rather than long-range dispersion forces. Therefore, the GBPM is relevant even for the BaTiO3 material for which dispersion forces are not expected to be important.

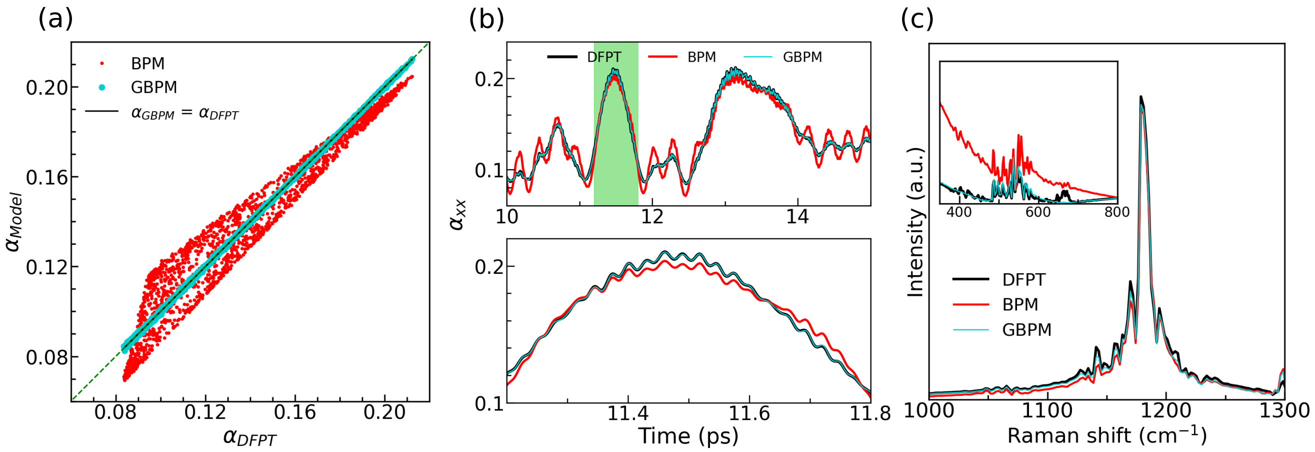


FIG. 1. $SO_2$ (a) $xx$ component of $\alpha_{BPM}$ (red circle) and $\alpha_{GBPM}$ (cyan circle) vs $\alpha_{DFPT}$. Linear fit of GBPM is shown in solid black line. Green dotted line represents $\alpha_{Model} = \alpha_{DFPT}$. (b) Top panel: Comparison of the trajectory of $\alpha_{xx}$ from DFPT (black), $\alpha_{BPM}$ (red) and $\alpha_{GBPM}$ (cyan). Bottom Panel: Magnified view of the region shaded in filled green in the first panel. (c) Raman spectra from DFPT (black), BPM (red) and GBPM (cyan). Inset shows the results in the lower-wavenumber region.

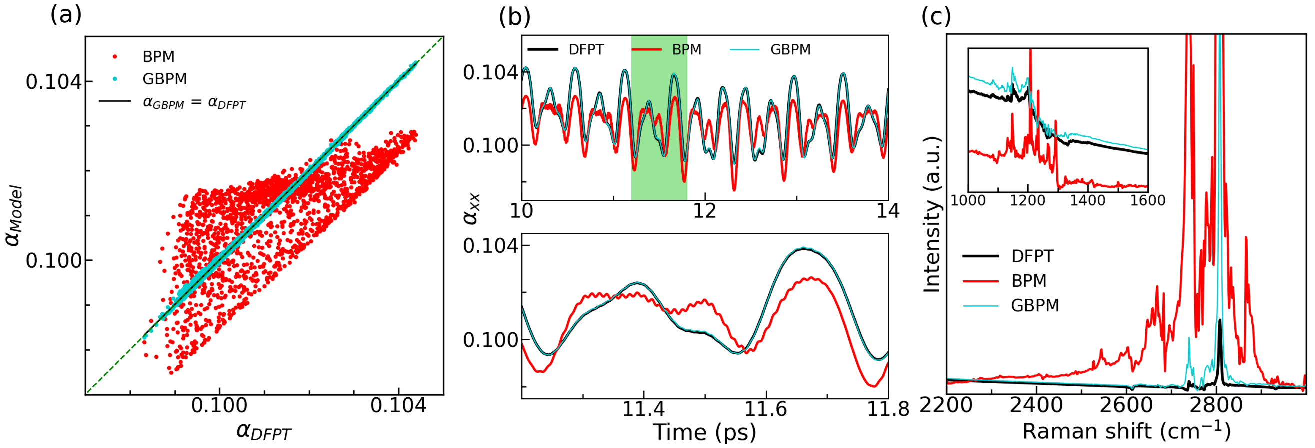


FIG. 2. $H_2S$ (a) $xx$ component of $\alpha_{BPM}$ (red circle) and $\alpha_{GBPM}$ (cyan circle) vs $\alpha_{DFPT}$. Linear fit of GBPM is shown in solid black line. Green dotted line represents $\alpha_{Model} = \alpha_{DFPT}$. (b) Top panel: Comparison of the trajectory of $\alpha_{xx}$ from DFPT (black), $\alpha_{BPM}$ (red) and $\alpha_{GBPM}$ (cyan). Bottom Panel: Magnified view of the region shaded in filled green in the first panel. (c) Raman spectra from DFPT (black), BPM (red) and GBPM (cyan). Inset shows the results in the lower-wavenumber region.

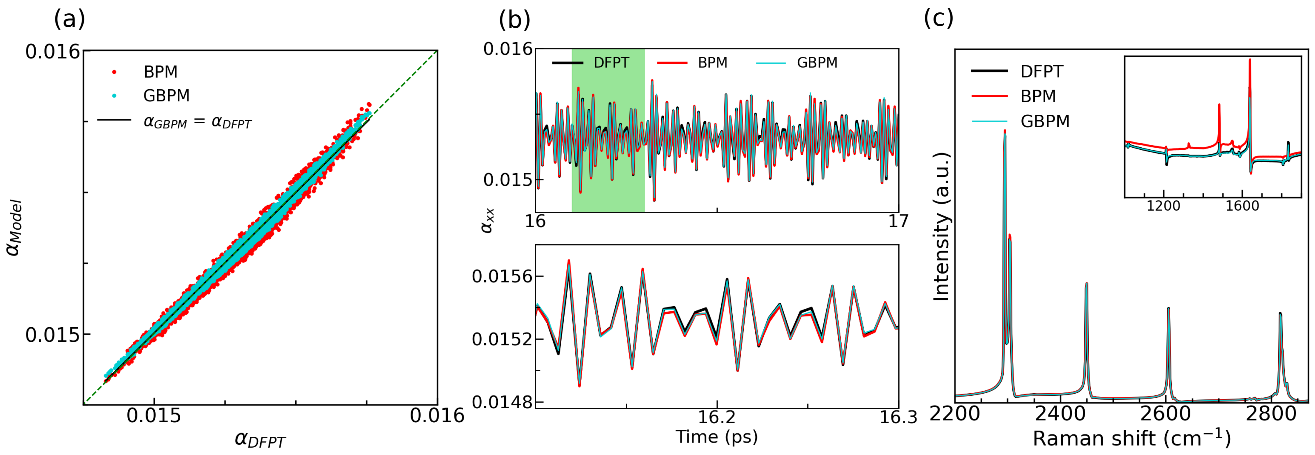


FIG. 3. $CH_4$ (a) $xx$ component of $\alpha_{BPM}$ (red circle) and $\alpha_{GBPM}$ (cyan circle) vs $\alpha_{DFPT}$. Linear fit of GBPM is shown in solid black line. Green dotted line represents $\alpha_{Model} = \alpha_{DFPT}$. (b) Top panel: Comparison of the trajectory of $\alpha_{xx}$ from DFPT (black), $\alpha_{BPM}$ (red) and $\alpha_{GBPM}$ (cyan) order. Bottom Panel: Magnified view of the region shaded in filled green in the first panel. (c) Raman spectra from DFPT (black), BPM (red) and GBPM (cyan). Inset shows the results in the lower-wavenumber region.

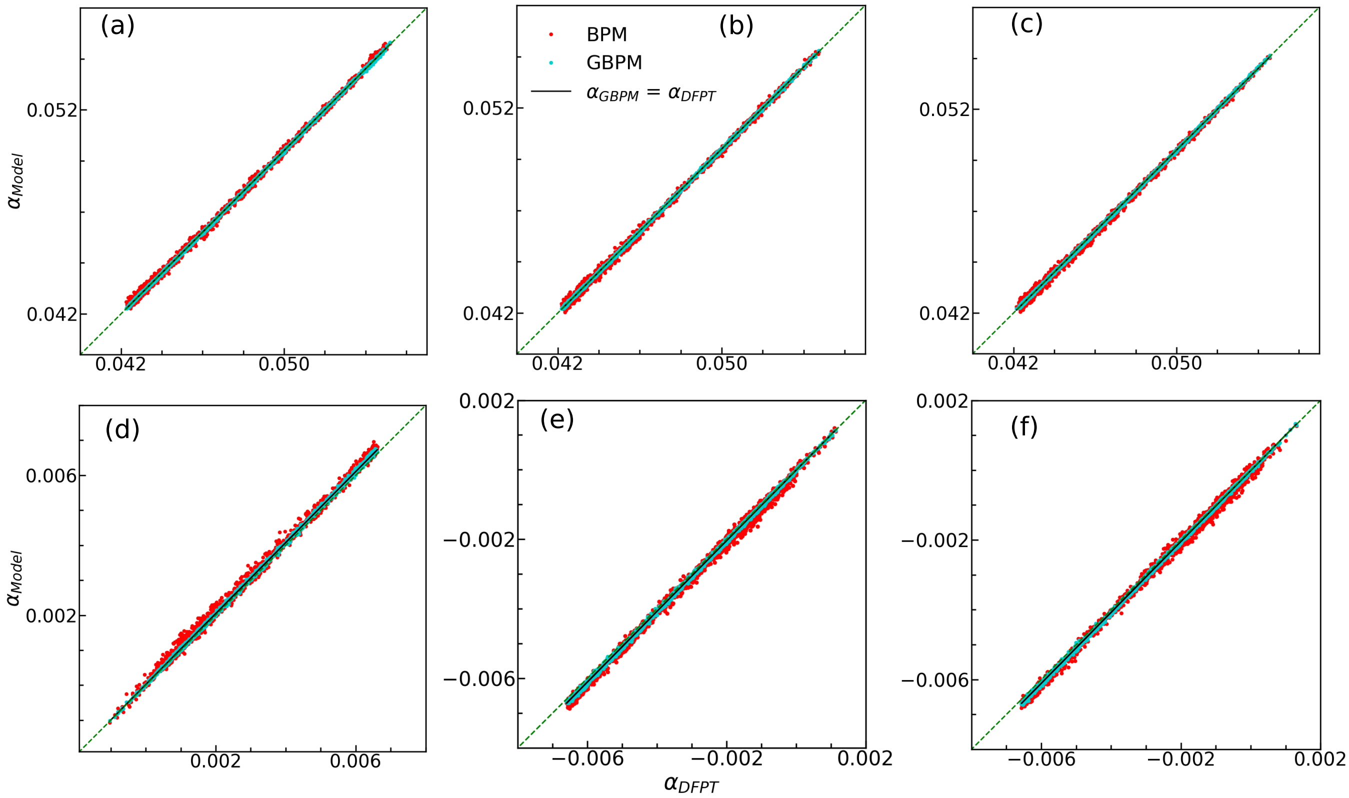


FIG. 4. $NH_3$: Comparison of (a) $\alpha_{xx}$, (b) $\alpha_{yy}$, (c) $\alpha_{zz}$, (d) $\alpha_{xy}$, (e) $\alpha_{xz}$ and (f) $\alpha_{yz}$ calculated using BPM (red) and GBPM (cyan) with DFPT. Linear fit of GBPM is shown in solid black line. Green dotted line represents $\alpha_{Model} = \alpha_{DFT}$.

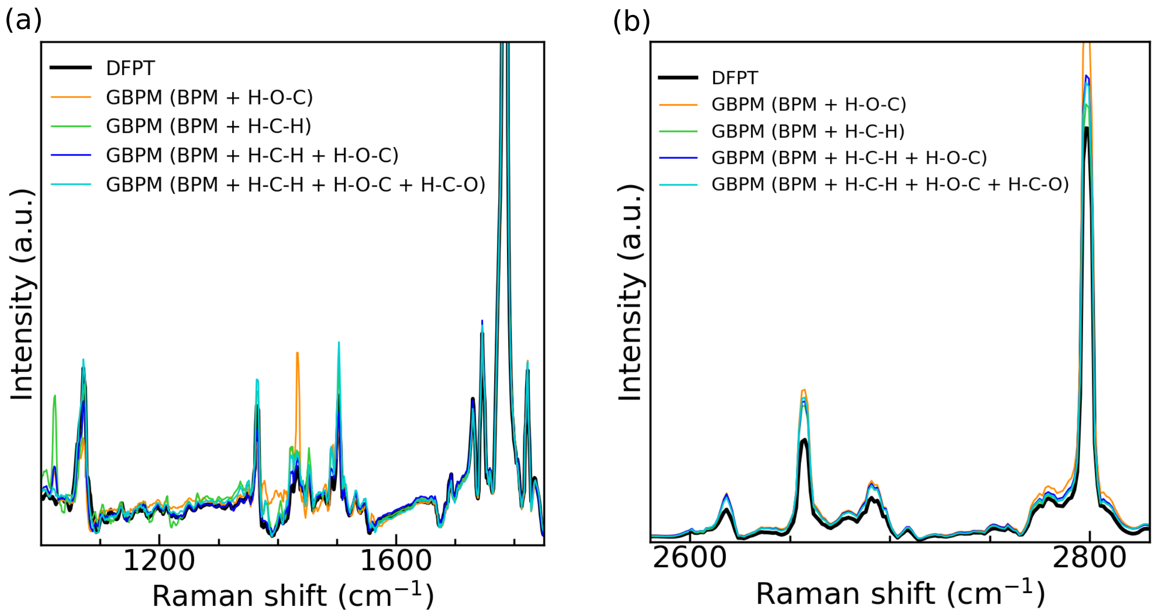


FIG. 5. Raman spectra of $CH_3OH$ calculated using different level of GBPM and DFPT in (a) lower and (b) higher wavenumber region.

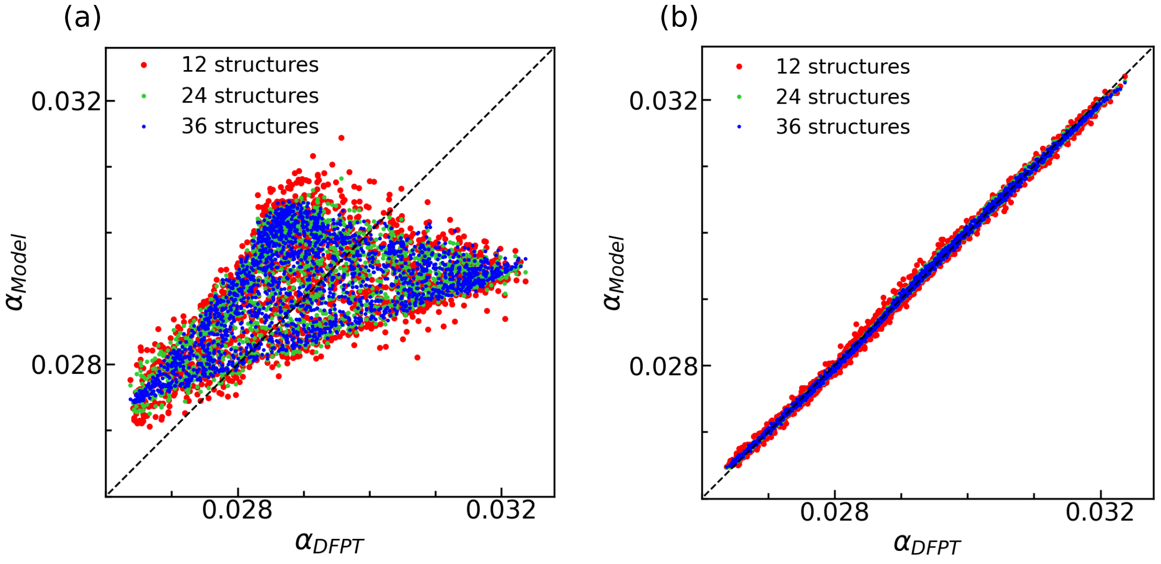


FIG. 6. $H_2O$: Comparison of the *xx* component of $\alpha$ calculated using (a) BPM and (b) GBPM with DFPT results considering different numbers of structures.

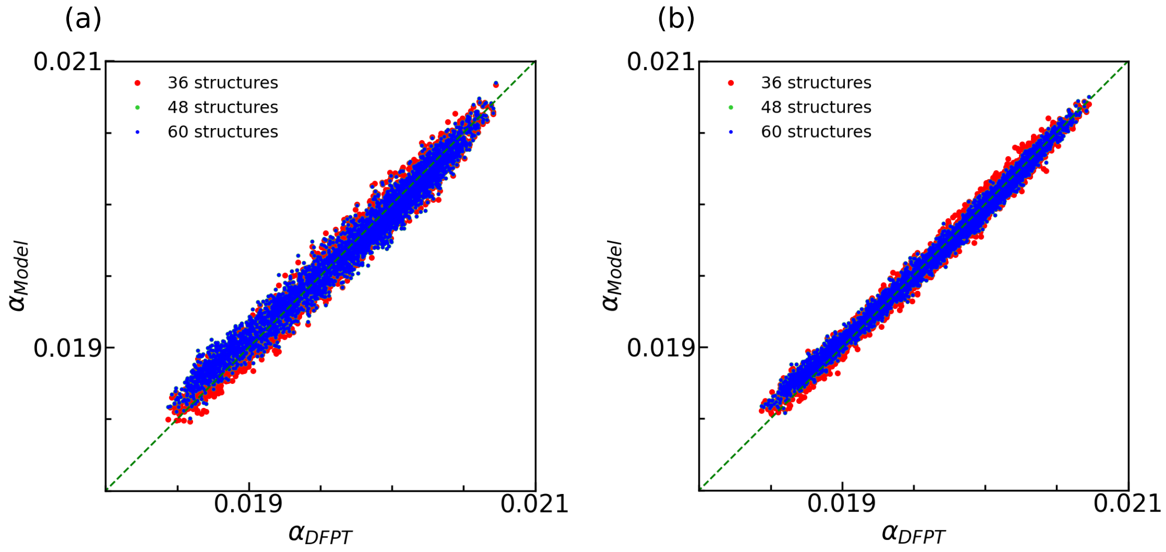


FIG. 7. $CH_3OH$: Comparison of the *xx* component of $\alpha$ calculated using (a) BPM and (b) GBPM with DFPT results considering different numbers of structures.

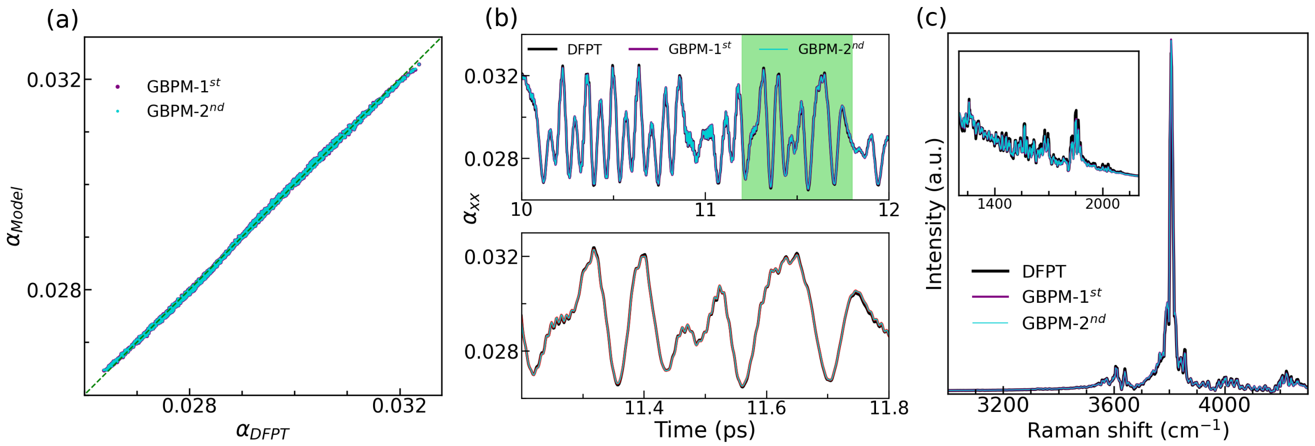


FIG. 8. $H_2O$: (a) *xx* component of $\alpha_{GBPM}$ (first- and second-order GBPM are represented by the purple and cyan circles, respectively) plotted vs that of $\alpha_{DFPT}$. (b) Top: comparison of the trajectory of $\alpha_{xx}$. Bottom: magnified view of the region in the first panel shaded in green. (c) Raman spectra generated using DFPT (black), first order and second order of GBPM. The inset shows the results in the lower-wavenumber region.

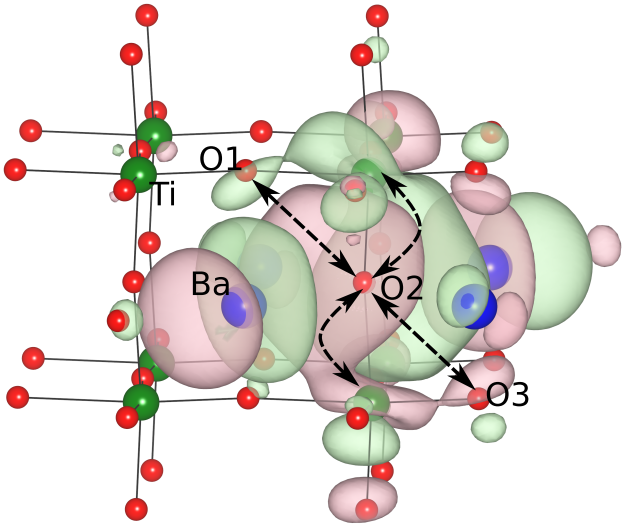


FIG. 9. Rhombohedral $BaTiO_3$: Maximally localized Wannier function of the O-$p$ orbital centered at O atom (marked as O2). Ba, Ti and O atoms are colored by blue, green and red, respectively.
